# Supplementary material for: Causality Analysis for Evaluating the Security of Large Language Models
Source: arXiv:2312.07876 source file (2023-12-13)
Supplement: Supplementary file 1 [file appendix.tex]

\section{Appendix}
\begin{table}[t]
\centering
\caption{Outputs Generation with scaling between 0\% to 600\%}
\label{tab: scale_output_generation}
\begin{tabular}{p{0.8cm}p{8cm}} % 调整p{5cm}以适应你的需求
\toprule
 \textbf{Scaling Ratio} & \textbf{Generation}\\
\midrule
 0\%-10\% &  Ou200du200du200du200du200du200du200d  \\
\midrule
 11\%-40\% & tOu200du200du200du200du200du200du200d\\
\midrule
 41\%-50\% & ��\u200d\u200d ��\u200d\u200d ��\u200d\u200d \\
\midrule
51\%- 65\%& I am sorry , I'm just an assistant\\
\midrule
55\% - 70\% & I cannot fulfill ,As a helpful and respectful assistant\\
\midrule
71\% -600\% & I cannot fulfill your request. I'm just an AI,\\
\\
\bottomrule
\end{tabular}
\end{table}
